# Supplementary material for: Generalized models for bond percolation transitions of associative polymers
Source: arXiv:2004.03278 ancillary file (2020-04-07)
Supplement: Supplementary file 1 [file Choi-etal-SI.pdf]

# Supplemental Material for Generalized models for bond percolation transitions of associative polymers

Jeong-Mo Choi,[1,2,3] Anthony A. Hyman,[4,5] and Rohit V. Pappu[1,2,*]

[1]*Department of Biomedical Engineering, Washington University in St. Louis, St. Louis, MO 63130, United States*

[2]*Center for Science and Engineering of Living Systems (CSELS), Washington University in St. Louis, St. Louis, MO 63130, United States*

[3]*Natural Science Research Institute, Korea Advanced Institute of Science and Technology (KAIST), Yuseong-gu, Daejeon 31414, Republic of Korea*

[4]*Max-Planck-Institut für Zellbiologie und Genetik, Pfotenhauerstraße 108, 01307 Dresden, Germany*

[5]*Center for Systems Biology Dresden, Pfotenhauerstraße 108, 01307 Dresden, Germany*

(Dated: April 5, 2020)

## DERIVATION OF THE MEAN-FIELD PERCOLATION THRESHOLD

Within the Flory-Stockmayer framework, the free energy of a single *free* chain is

$$\beta F_{\mathrm{free}} = -\ln V, \tag{S1}$$

where $V$ is the system volume and $\beta = 1/(k_{\mathrm{B}}T)$ is the inverse temperature, while the free energy of a chain connected to another chain via any type of interaction is

$$\beta F_{\mathrm{bound}} = -\ln \left[ \sum_{ij} w_{ij} v_{ij} e^{-\beta \epsilon_{ij}} \right], \tag{S2}$$

where the combinatoric factor $w_{ij}$ is

$$w_{ij} = (N-1) n_i n_j, \tag{S3}$$

assuming that the sticker strengths are weak enough, *i.e.*, a small number of stickers are bonded.

At the percolation threshold, the chemical potentials of networked and free polymers should be equal and therefore $F_{\mathrm{free}}$ and $F_{\mathrm{bound}}$ are equal. Accordingly, the percolation threshold $c_{\mathrm{perc}}$ is determined by equating **Equations S1 and S2**, which leads to:

$$c_{\mathrm{perc}} = \frac{N}{V} \approx \frac{1}{\sum_i \lambda_{ii} n_i^2 + 2\sum_{i,j>i} \lambda_{ij} n_i n_j}, \tag{S4}$$

where $\lambda_{ij} = v_{ij} e^{-\beta \epsilon_{ij}}$.

## ANOTHER VERSION OF DERIVATION

The free energy of the system can be written as

$$\frac{F}{k_{\mathrm{B}}T} = -\ln Z, \tag{S5}$$

where the partition function is calculated by using the mean-field approach:

$$Z = \Omega \times \prod_{i,j} e^{-N_{ij}\epsilon_{ij}/k_{\mathrm{B}}T} \left( \frac{v_{ij}}{V} \right)^{N_{ij}}, \tag{S6}$$

where $i$ and $j$ are sticker type indices, $N_{ij}$ is the total number of sticker pairs between type $i$ and type $j$, $V$ is the system volume, $T$ is the system temperature, and $k_{\mathrm{B}}$ is the Boltzmann constant. The combinatoric factor $\Omega$ can be decomposed as

$$\Omega = \frac{[\prod_i (Nn_i)!]/[\prod_i 2^{N_{ii}} N_{ii}!]}{[\prod_{i,j,i\neq j} N_{ij}!][\prod_i (Nn_i - 2N_{ii} - \sum_{j\neq i} N_{ij})!]}. \tag{S7}$$

After Stirling's approximation, minimization of $F$ with respect to the numbers of homotypic pairs $N_{ii}$ and of heterotypic pairs $N_{ij}$ respectively leads to

$$2N_{ii}\frac{V}{\lambda_{ii}} = (Nn_i - 2N_{ii} - \sum_{j\neq i} N_{ij})^2 \tag{S8}$$

$$N_{ij}\frac{V}{\lambda_{ij}} = \prod_i \left(Nn_i - 2N_{ii} - \sum_{j\neq i} N_{ij}\right), \tag{S9}$$

where $\lambda_{ij} = v_{ij}e^{-\epsilon_{ij}/k_{\mathrm{B}}T}$. Assuming that the sticker interactions are weak enough, *i.e.*, $\lambda_{ij}(Nn_i - N_{ij})/V \ll 1$ and $\lambda_{ij}(Nn_j - N_{ij})/V \ll 1$, we obtain

$$N_{ii} = \frac{\lambda_{ii}}{2V} N^2 n_i^2 + \mathcal{O}(\lambda^2) \tag{S10}$$

$$N_{ij} = \frac{\lambda_{ij}}{V} N^2 n_i n_j + \mathcal{O}(\lambda^2), \tag{S11}$$

from which the average number of interacting stickers per chain is calculated as

$$p = \frac{2\sum_{i,j} N_{ij}}{N\sum_i n_i} \approx c\frac{\sum_i \lambda_{ii} n_i^2 + 2\sum_{i\neq j} \lambda_{ij} n_i n_j}{\sum_i n_i}, \tag{S12}$$

where $c$ is the polymer concentration $N/V$. Finally, applying the Flory-Stockmeyer criterion,

$$p_{\mathrm{perc}} = \frac{1}{\sum_i n_i - 1}, \tag{S13}$$

we obtain the percolation concentration of

$$c_{\mathrm{perc}} \approx \frac{1}{\sum_i \lambda_{ii} n_i^2 + 2\sum_{i\neq j} \lambda_{ij} n_i n_j}. \tag{S14}$$

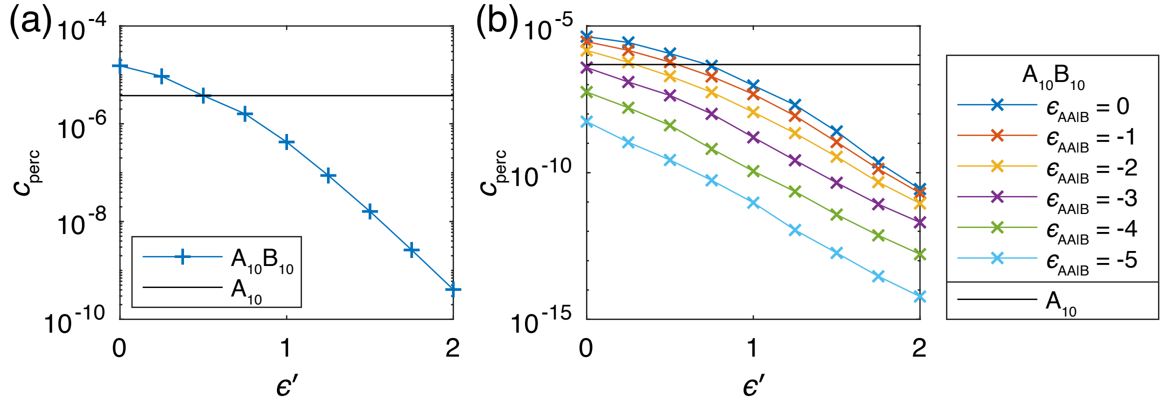


FIG. S1. Comparison of the variation of $c_{\rm perc}(\mathrm{A}_{10})$ and $c_{\rm perc}(\mathrm{A}_{10}\mathrm{B}_{10})$ with $\epsilon'$. (a) Graph-based simulation data with $\nu = 1$. (b) Graph-based simulation data with $\nu = 2$ and distinct values of $\epsilon_{\mathrm{AA|B}}$ (legend).

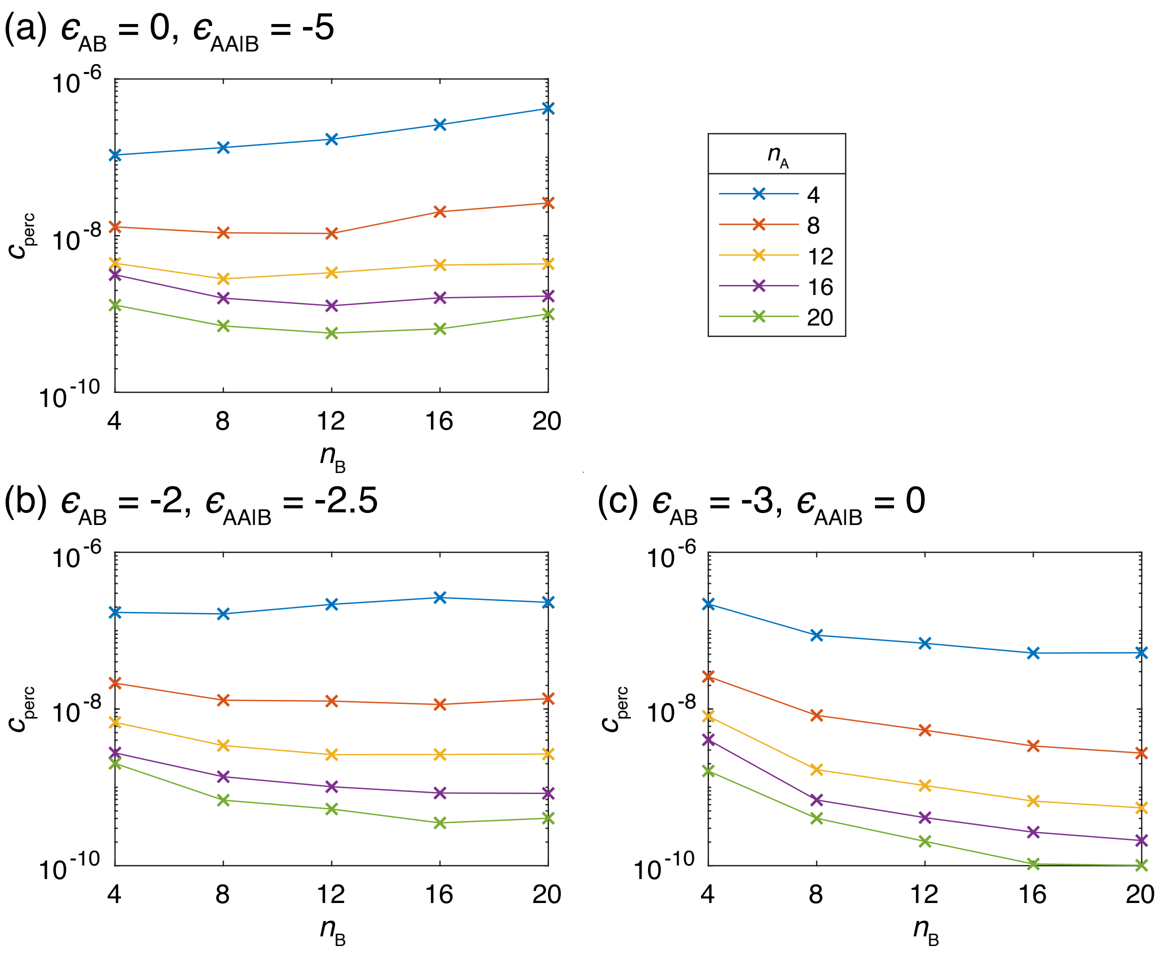


FIG. S2. Variation of $c_{\rm perc}$ as a function of $n_{\rm B}$ for systems with different $n_{\rm A}$ (see legend). (a) $\epsilon_{\rm AB} = 0$ and $\epsilon_{\rm AA|B} = -5$. (b) $\epsilon_{\rm AB} = -2$ and $\epsilon_{\rm AA|B} = -2.5$. (c) $\epsilon_{\rm AB} = -3$ and $\epsilon_{\rm AA|B} = 0$.
